# Supplementary material for: Molecular Origins of Exciton Condensation in Van der Waals Heterostructure Bilayers
Source: arXiv:2411.03164 source file (2024-11-05)
Supplement: Supplementary file 1 [file SI.pdf]

# Supporting Information: Molecular Origins of Exciton Condensation in Van der Waals Heterostructure Bilayers

Lillian I. Payne Torres, Anna O. Schouten, and David A. Mazziotti*

*Department of Chemistry and The James Franck Institute, The University of Chicago, Chicago, IL 60637*

E-mail: damazz@uchicago.edu

Table 1: $2 \times 2$ $MoSe_2$-$WSe_2$

| Atom | X | Y | Z |
|---|---|---|---|
| Mo | 0.00000 | 1.91869 | 7.10596 |
| Mo | -1.66163 | 4.79673 | 7.10596 |
| Mo | 3.32327 | 1.91869 | 7.10596 |
| Mo | 1.66163 | 4.79673 | 7.10596 |
| W | 1.66163 | 0.95935 | 0.00000 |
| W | 0.00000 | 3.83738 | 0.00000 |
| W | 4.98491 | 0.95935 | 0.00000 |
| W | 3.32327 | 3.83738 | 0.00000 |
| Se | 0.00000 | 1.91869 | 1.68443 |
| Se | -1.66163 | 4.79673 | 1.68443 |
| Se | 3.32327 | 1.91869 | 1.68443 |
| Se | 1.66163 | 4.79673 | 1.68443 |
| Se | 1.66163 | 0.95935 | 5.42989 |
| Se | 0.00000 | 3.83738 | 5.42989 |
| Se | 4.98491 | 0.95935 | 5.42989 |
| Se | 3.32327 | 3.83738 | 5.42989 |
| Se | 1.66163 | 0.95935 | 8.78170 |
| Se | 0.00000 | 3.83738 | 8.78170 |
| Se | 4.98491 | 0.95935 | 8.78170 |
| Se | 3.32327 | 3.83738 | 8.78170 |
| Se | -1.66163 | 0.95935 | 5.42989 |
| Se | -1.66163 | 0.95935 | 8.78170 |
| Se | -3.32327 | 3.83738 | 5.42989 |
| Se | -3.32327 | 3.83738 | 8.78170 |
| Se | -1.66163 | 6.71542 | 5.42989 |
| Se | -1.66163 | 6.71542 | 8.78170 |
| Se | 1.66163 | 6.71542 | 5.42989 |
| Se | 1.66163 | 6.71542 | 8.78170 |
| Se | 1.66163 | -0.95935 | -1.68443 |
| Se | 1.66163 | -0.95935 | 1.68443 |

| Atom | X | Y | Z |
|---|---|---|---|
| Se | 0.00000 | 1.91869 | -1.68443 |
| Se | 3.32327 | 1.91869 | -1.68443 |
| Se | -1.66163 | 4.79673 | -1.68443 |
| Se | 1.66163 | 4.79673 | -1.68443 |
| Se | 4.98491 | -0.95935 | -1.68443 |
| Se | 4.98491 | -0.95935 | 1.68443 |
| Se | 6.64654 | 1.91869 | -1.68443 |
| Se | 6.64654 | 1.91869 | 1.68443 |
| Se | 4.98491 | 4.79673 | -1.68443 |
| Se | 4.98491 | 4.79673 | 1.68443 |
| H | -3.07009 | 4.52731 | 1.21139 |
| H | 4.35981 | -0.21659 | 4.71819 |
| H | 5.45321 | -0.39541 | 8.30690 |
| H | -1.03654 | -0.21659 | 4.71819 |
| H | -2.12994 | -0.39541 | 8.30690 |
| H | -4.02911 | 4.96670 | 4.71819 |
| H | -4.73068 | 4.10920 | 8.30690 |
| H | -2.99258 | 6.76204 | 4.71819 |
| H | -2.60074 | 7.79836 | 8.30690 |
| H | 0.33069 | 6.76204 | 4.71819 |
| H | 0.72253 | 7.79836 | 8.30690 |
| H | 2.99204 | -1.00327 | -2.39731 |
| H | 2.59918 | -2.04440 | 1.21139 |
| H | -2.36488 | 3.66653 | -2.39731 |
| H | 6.31531 | -1.00327 | -2.39731 |
| H | 5.92245 | -2.04440 | 1.21139 |
| H | 7.34978 | 0.78849 | -2.39731 |
| H | 8.05500 | 1.64928 | 1.21139 |
| H | 5.68815 | 3.66653 | -2.39731 |
| H | 6.39336 | 4.52731 | 1.21139 |

Table 2: $3 \times 3$ $MoSe_2$-$WSe_2$

| Atom | X | Y | Z |
|---|---|---|---|
| Mo | 0.00000 | 1.91869 | 54.32685 |
| Mo | -1.66163 | 4.79673 | 54.32685 |
| Mo | -3.32327 | 7.67476 | 54.32685 |
| Mo | 3.32327 | 1.91869 | 54.32685 |
| Mo | 1.66163 | 4.79673 | 54.32685 |
| Mo | 0.00000 | 7.67476 | 54.32685 |
| Mo | 6.64654 | 1.91869 | 54.32685 |
| Mo | 4.98491 | 4.79673 | 54.32685 |
| Mo | 3.32327 | 7.67476 | 54.32685 |
| W | 1.66163 | 0.95935 | 61.43281 |
| W | 0.00000 | 3.83738 | 61.43281 |
| W | -1.66163 | 6.71542 | 61.43281 |
| W | 4.98491 | 0.95935 | 61.43281 |
| W | 3.32327 | 3.83738 | 61.43281 |
| W | 1.66163 | 6.71542 | 61.43281 |
| W | 8.30818 | 0.95935 | 61.43281 |
| W | 6.64654 | 3.83738 | 61.43281 |
| W | 4.98491 | 6.71542 | 61.43281 |
| Se | 0.00000 | 1.91869 | 59.74838 |
| Se | -1.66163 | 4.79673 | 59.74838 |
| Se | -3.32327 | 7.67476 | 59.74838 |
| Se | 3.32327 | 1.91869 | 59.74838 |
| Se | 1.66163 | 4.79673 | 59.74838 |
| Se | 0.00000 | 7.67476 | 59.74838 |
| Se | 6.64654 | 1.91869 | 59.74838 |
| Se | 4.98491 | 4.79673 | 59.74838 |
| Se | 3.32327 | 7.67476 | 59.74838 |
| Se | 1.66163 | 0.95935 | 56.00292 |
| Se | 0.00000 | 3.83738 | 56.00292 |
| Se | -1.66163 | 6.71542 | 56.00292 |
| Se | 4.98491 | 0.95935 | 56.00292 |
| Se | 3.32327 | 3.83738 | 56.00292 |
| Se | 1.66163 | 6.71542 | 56.00292 |
| Se | 8.30818 | 0.95935 | 56.00292 |
| Se | 6.64654 | 3.83738 | 56.00292 |
| Se | 4.98491 | 6.71542 | 56.00292 |
| Se | 1.66163 | 0.95935 | 52.65111 |
| Se | 0.00000 | 3.83738 | 52.65111 |
| Se | -1.66163 | 6.71542 | 52.65111 |
| Se | 4.98491 | 0.95935 | 52.65111 |
| Se | 3.32327 | 3.83738 | 52.65111 |
| Se | 1.66163 | 6.71542 | 52.65111 |
| Se | 8.30818 | 0.95935 | 52.65111 |
| Se | 6.64654 | 3.83738 | 52.65111 |
| Se | 4.98491 | 6.71542 | 52.65111 |
| Se | -1.66163 | 0.95935 | 52.65111 |
| Se | -1.66163 | 0.95935 | 56.00292 |
| Se | -3.32327 | 3.83738 | 52.65111 |
| Se | -3.32327 | 3.83738 | 56.00292 |
| Se | -4.98491 | 6.71542 | 52.65111 |
| Se | -4.98491 | 6.71542 | 56.00292 |
| Se | -3.32327 | 9.59346 | 52.65111 |
| Se | -3.32327 | 9.59346 | 56.00292 |

| Atom | X | Y | Z |
|---|---|---|---|
| Se | 0.00000 | 9.59346 | 52.65111 |
| Se | 0.00000 | 9.59346 | 56.00292 |
| Se | 3.32327 | 9.59346 | 52.65111 |
| Se | 3.32327 | 9.59346 | 56.00292 |
| Se | 1.66163 | -0.95935 | 59.74838 |
| Se | 1.66163 | -0.95935 | 63.11724 |
| Se | 0.00000 | 1.91869 | 63.11724 |
| Se | 3.32327 | 1.91869 | 63.11724 |
| Se | -1.66163 | 4.79673 | 63.11724 |
| Se | 1.66163 | 4.79673 | 63.11724 |
| Se | -3.32327 | 7.67476 | 63.11724 |
| Se | 0.00000 | 7.67476 | 63.11724 |
| Se | 4.98491 | -0.95935 | 59.74838 |
| Se | 4.98491 | -0.95935 | 63.11724 |
| Se | 6.64654 | 1.91869 | 63.11724 |
| Se | 4.98491 | 4.79673 | 63.11724 |
| Se | 3.32327 | 7.67476 | 63.11724 |
| Se | 8.30818 | -0.95935 | 59.74838 |
| Se | 8.30818 | -0.95935 | 63.11724 |
| Se | 9.96981 | 1.91869 | 59.74838 |
| Se | 9.96981 | 1.91869 | 63.11724 |
| Se | 8.30818 | 4.79673 | 59.74838 |
| Se | 8.30818 | 4.79673 | 63.11724 |
| Se | 6.64654 | 7.67476 | 59.74838 |
| Se | 6.64654 | 7.67476 | 63.11724 |
| H | -4.02651 | 6.54457 | 59.03550 |
| H | 8.77658 | -0.39540 | 55.52819 |
| H | 7.68302 | -0.21643 | 51.93918 |
| H | -1.17892 | 1.23804 | 51.24775 |
| H | -3.06908 | 1.23107 | 55.52819 |
| H | -2.84056 | 4.11608 | 51.24775 |
| H | -4.73072 | 4.10910 | 55.52819 |
| H | -4.50219 | 6.99411 | 51.24775 |
| H | -5.45331 | 5.36067 | 55.52819 |
| H | -1.99245 | 9.63994 | 51.93918 |
| H | -2.38423 | 10.67648 | 55.52819 |
| H | 0.00000 | 9.03607 | 51.24775 |
| H | 0.93904 | 10.67648 | 55.52819 |
| H | 3.32327 | 9.03607 | 51.24775 |
| H | 2.38423 | 10.67648 | 55.52819 |
| H | 1.66163 | -0.39836 | 58.34646 |
| H | 2.59918 | -2.04440 | 62.64420 |
| H | -4.73173 | 7.40535 | 62.64420 |
| H | 4.98491 | -0.39836 | 58.34646 |
| H | 5.92245 | -2.04440 | 62.64420 |
| H | 9.63858 | -1.00327 | 59.03550 |
| H | 9.24572 | -2.04440 | 62.64420 |
| H | 10.67305 | 0.78849 | 59.03550 |
| H | 11.37827 | 1.64928 | 62.64420 |
| H | 7.82235 | 4.51623 | 58.34646 |
| H | 7.82235 | 4.51623 | 64.51916 |
| H | 6.16071 | 7.39427 | 58.34646 |
| H | 7.11745 | 9.02923 | 62.64420 |

Table 3: $2 \times 2$ $MoS_2$-$WS_2$

| Atom | X | Y | Z |
|---|---|---|---|
| W | 1.59000 | 0.91799 | 3.12500 |
| W | 0.00000 | 3.67195 | 3.12500 |
| W | 4.77000 | 0.91799 | 3.12500 |
| W | 3.18000 | 3.67195 | 3.12500 |
| S | 0.00000 | 1.83597 | 4.68750 |
| S | -1.59000 | 4.58993 | 4.68750 |
| S | 3.18000 | 1.83597 | 4.68750 |
| S | 1.59000 | 4.58993 | 4.68750 |
| S | 0.00000 | 1.83597 | 1.56250 |
| S | -1.59000 | 4.58993 | 1.56250 |
| S | 3.18000 | 1.83597 | 1.56250 |
| S | 1.59000 | 4.58993 | 1.56250 |
| S | 1.59000 | -0.91799 | 1.56250 |
| S | 1.59000 | -0.91799 | 4.68750 |
| S | 4.77000 | -0.91799 | 1.56250 |
| S | 4.77000 | -0.91799 | 4.68750 |
| S | 6.36000 | 1.83597 | 1.56250 |
| S | 6.36000 | 1.83597 | 4.68750 |
| S | 4.77000 | 4.58993 | 1.56250 |
| S | 4.77000 | 4.58993 | 4.68750 |
| S | 1.58030 | 6.38762 | 11.44518 |
| S | 1.58030 | 6.38762 | 8.43288 |
| Mo | 1.58030 | 4.56262 | 9.93898 |
| S | 3.16080 | 3.65012 | 11.44518 |
| S | -1.58070 | 6.38762 | 11.44518 |
| S | -1.58070 | 6.38762 | 8.43288 |
| S | 3.16080 | 3.65012 | 8.43288 |
| Mo | 3.16080 | 1.82512 | 9.93898 |
| Mo | -1.58070 | 4.56262 | 9.93898 |
| S | 4.74130 | 0.91262 | 8.43288 |

| Atom | X | Y | Z |
|---|---|---|---|
| S | -0.00020 | 3.65012 | 11.44518 |
| S | 4.74130 | 0.91262 | 11.44518 |
| S | -0.00020 | 3.65012 | 8.43288 |
| Mo | -0.00020 | 1.82512 | 9.93898 |
| S | 1.58030 | 0.91262 | 11.44518 |
| S | -3.16120 | 3.65012 | 8.43288 |
| S | -3.16120 | 3.65012 | 11.44518 |
| S | 1.58030 | 0.91262 | 8.43288 |
| S | -1.58070 | 0.91262 | 11.44518 |
| S | -1.58070 | 0.91262 | 8.43288 |
| H | -2.85281 | 4.33418 | 4.25218 |
| H | -2.23721 | 3.57691 | 0.92648 |
| H | 0.38910 | -0.97198 | 0.92648 |
| H | 0.73710 | -1.88374 | 4.25218 |
| H | 3.56910 | -0.97198 | 0.92648 |
| H | 3.91710 | -1.88374 | 4.25218 |
| H | 5.93929 | 1.59307 | 0.29222 |
| H | 6.76992 | 3.05747 | 4.25219 |
| H | 4.34929 | 4.34703 | 0.29222 |
| H | 6.03281 | 4.33418 | 4.25218 |
| H | 0.71885 | 7.34179 | 11.00125 |
| H | 1.58030 | 5.92112 | 7.15539 |
| H | -0.71925 | 7.34179 | 11.00125 |
| H | -0.37719 | 6.45572 | 7.80318 |
| H | 4.19852 | -0.16370 | 7.80318 |
| H | 5.13691 | -0.31050 | 11.00124 |
| H | -2.75720 | 3.88337 | 7.15539 |
| H | -1.17670 | 1.14587 | 7.15539 |
| H | -3.55681 | 2.42700 | 11.00124 |
| H | -2.83775 | 1.18157 | 11.00124 |

Table 4: $3 \times 3$ $MoS_2$-$WS_2$

| Atom | X | Y | Z |
|---|---|---|---|
| W | 1.59000 | 0.91799 | 3.12500 |
| W | 0.00000 | 3.67195 | 3.12500 |
| W | -1.59000 | 6.42591 | 3.12500 |
| W | 4.77000 | 0.91799 | 3.12500 |
| W | 3.18000 | 3.67195 | 3.12500 |
| W | 1.59000 | 6.42591 | 3.12500 |
| W | 7.95000 | 0.91799 | 3.12500 |
| W | 6.36000 | 3.67195 | 3.12500 |
| W | 4.77000 | 6.42591 | 3.12500 |
| S | 0.00000 | 1.83597 | 4.68750 |
| S | -1.59000 | 4.58993 | 4.68750 |
| S | -3.18000 | 7.34390 | 4.68750 |
| S | 3.18000 | 1.83597 | 4.68750 |
| S | 1.59000 | 4.58993 | 4.68750 |
| S | 0.00000 | 7.34390 | 4.68750 |
| S | 6.36000 | 1.83597 | 4.68750 |
| S | 4.77000 | 4.58993 | 4.68750 |
| S | 3.18000 | 7.34390 | 4.68750 |
| S | 0.00000 | 1.83597 | 1.56250 |
| S | -1.59000 | 4.58993 | 1.56250 |
| S | -3.18000 | 7.34390 | 1.56250 |
| S | 3.18000 | 1.83597 | 1.56250 |
| S | 1.59000 | 4.58993 | 1.56250 |
| S | 0.00000 | 7.34390 | 1.56250 |
| S | 6.36000 | 1.83597 | 1.56250 |
| S | 4.77000 | 4.58993 | 1.56250 |
| S | 3.18000 | 7.34390 | 1.56250 |
| S | 1.59000 | -0.91799 | 1.56250 |
| S | 1.59000 | -0.91799 | 4.68750 |
| S | 4.77000 | -0.91799 | 1.56250 |
| S | 4.77000 | -0.91799 | 4.68750 |
| S | 7.95000 | -0.91799 | 1.56250 |
| S | 7.95000 | -0.91799 | 4.68750 |
| S | 9.54000 | 1.83597 | 1.56250 |
| S | 9.54000 | 1.83597 | 4.68750 |
| S | 7.95000 | 4.58993 | 1.56250 |
| S | 7.95000 | 4.58993 | 4.68750 |
| S | 6.36000 | 7.34390 | 1.56250 |
| S | 6.36000 | 7.34390 | 4.68750 |
| S | 3.14712 | 9.13301 | 11.44493 |
| S | 3.14712 | 9.13301 | 8.43263 |
| Mo | 3.14712 | 7.30801 | 9.93873 |
| S | 4.72762 | 6.39551 | 8.43263 |
| S | 4.72762 | 6.39551 | 11.44493 |
| S | -0.01388 | 9.13301 | 11.44493 |
| S | -0.01388 | 9.13301 | 8.43263 |
| Mo | -0.01388 | 7.30801 | 9.93873 |
| Mo | 4.72762 | 4.57051 | 9.93873 |
| S | 6.30812 | 3.65801 | 8.43263 |
| S | -3.17488 | 9.13301 | 8.43263 |
| S | -3.17488 | 9.13301 | 11.44493 |
| S | 6.30812 | 3.65801 | 11.44493 |
| S | 1.56662 | 6.39551 | 8.43263 |
| S | 1.56662 | 6.39551 | 11.44493 |
| Mo | -3.17488 | 7.30801 | 9.93873 |
| Mo | 1.56662 | 4.57051 | 9.93873 |
| Mo | 6.30812 | 1.83301 | 9.93873 |
| S | 3.14712 | 3.65801 | 8.43263 |
| S | -1.59438 | 6.39551 | 11.44493 |
| S | -1.59438 | 6.39551 | 8.43263 |
| S | 7.88862 | 0.92051 | 8.43263 |
| S | 7.88862 | 0.92051 | 11.44493 |
| S | 3.14712 | 3.65801 | 11.44493 |
| Mo | 3.14712 | 1.83301 | 9.93873 |
| Mo | -1.59438 | 4.57051 | 9.93873 |
| S | -4.75538 | 6.39551 | 11.44493 |
| S | -0.01388 | 3.65801 | 11.44493 |
| S | -4.75538 | 6.39551 | 8.43263 |
| S | 4.72762 | 0.92051 | 11.44493 |
| S | -0.01388 | 3.65801 | 8.43263 |
| S | 4.72762 | 0.92051 | 8.43263 |
| Mo | -0.01388 | 1.83301 | 9.93873 |
| S | -3.17488 | 3.65801 | 11.44493 |
| S | -3.17488 | 3.65801 | 8.43263 |
| S | 1.56662 | 0.92051 | 8.43263 |
| S | 1.56662 | 0.92051 | 11.44493 |
| S | -1.59438 | 0.92051 | 11.44493 |
| S | -1.59438 | 0.92051 | 8.43263 |
| H | -4.44281 | 7.08815 | 4.25218 |
| H | -3.82721 | 6.33089 | 0.92648 |
| H | 0.38910 | -0.97198 | 0.92648 |
| H | 0.73710 | -1.88374 | 4.25218 |
| H | 3.56910 | -0.97198 | 0.92648 |
| H | 3.91710 | -1.88374 | 4.25218 |
| H | 6.74910 | -0.97198 | 0.92648 |
| H | 7.09710 | -1.88374 | 4.25218 |
| H | 9.11929 | 1.59307 | 0.29222 |
| H | 10.80281 | 1.58022 | 4.25218 |
| H | 7.52929 | 4.34703 | 0.29222 |
| H | 8.35992 | 5.81143 | 4.25219 |
| H | 5.93929 | 7.10100 | 0.29222 |
| H | 7.62281 | 7.08815 | 4.25218 |
| H | 4.00857 | 10.08718 | 11.00100 |
| H | 3.14712 | 8.66651 | 7.15514 |
| H | -0.87533 | 10.08718 | 11.00100 |
| H | -1.21739 | 9.20111 | 7.80293 |
| H | -4.37839 | 9.20111 | 7.80293 |
| H | -4.03633 | 10.08718 | 11.00100 |
| H | 7.34584 | -0.15581 | 7.80293 |
| H | 8.28423 | -0.30261 | 11.00099 |
| H | -6.01243 | 6.66446 | 11.00099 |
| H | -5.41611 | 7.40373 | 7.80293 |
| H | -3.57049 | 2.43489 | 11.00099 |
| H | -2.77088 | 3.89126 | 7.15514 |
| H | -2.85143 | 1.18946 | 11.00099 |
| H | -1.19038 | 1.15376 | 7.15514 |

Table 5: $2 \times 2$ $MoSe_2$-$WS_2$

| Atom | X | Y | Z |
|---|---|---|---|
| Mo | 0.00000 | 1.89833 | 3.23000 |
| Mo | -1.64400 | 4.74582 | 3.23000 |
| Mo | 3.28800 | 1.89833 | 3.23000 |
| Mo | 1.64400 | 4.74582 | 3.23000 |
| Se | 1.64400 | 0.94916 | 4.89668 |
| Se | 0.00000 | 3.79665 | 4.89668 |
| Se | 4.93200 | 0.94916 | 4.89668 |
| Se | 3.28800 | 3.79665 | 4.89668 |
| Se | 1.64400 | 0.94916 | 1.56332 |
| Se | 0.00000 | 3.79665 | 1.56332 |
| Se | 4.93200 | 0.94916 | 1.56332 |
| Se | 3.28800 | 3.79665 | 1.56332 |
| Se | -1.64400 | 0.94916 | 1.56332 |
| Se | -1.64400 | 0.94916 | 4.89668 |
| Se | -3.28800 | 3.79665 | 1.56332 |
| Se | -3.28800 | 3.79665 | 4.89668 |
| Se | -1.64400 | 6.64415 | 1.56332 |
| Se | -1.64400 | 6.64415 | 4.89668 |
| Se | 1.64400 | 6.64415 | 1.56332 |
| Se | 1.64400 | 6.64415 | 4.89668 |
| S | 1.70467 | -0.84065 | 8.64082 |
| S | 1.70467 | -0.84065 | 11.76582 |
| W | 1.70467 | 0.99535 | 10.20332 |
| S | 0.11467 | 1.91335 | 11.76582 |
| S | 0.11467 | 1.91335 | 8.64082 |
| S | 4.88467 | -0.84065 | 8.64082 |
| S | 4.88467 | -0.84065 | 11.76582 |
| W | 0.11467 | 3.74925 | 10.20332 |
| W | 4.88467 | 0.99535 | 10.20332 |
| S | 3.29467 | 1.91335 | 8.64082 |

| Atom | X | Y | Z |
|---|---|---|---|
| S | -1.47533 | 4.66725 | 11.76582 |
| S | -1.47533 | 4.66725 | 8.64082 |
| S | 3.29467 | 1.91335 | 11.76582 |
| W | 3.29467 | 3.74925 | 10.20332 |
| S | 6.47467 | 1.91335 | 11.76582 |
| S | 6.47467 | 1.91335 | 8.64082 |
| S | 1.70467 | 4.66725 | 8.64082 |
| S | 1.70467 | 4.66725 | 11.76582 |
| S | 4.88467 | 4.66725 | 8.64082 |
| S | 4.88467 | 4.66725 | 11.76582 |
| H | 5.40295 | -0.40530 | 4.42367 |
| H | 4.30481 | -0.22493 | 0.85042 |
| H | -1.15812 | 1.22968 | 0.16142 |
| H | -2.11495 | -0.40530 | 4.42367 |
| H | -2.80212 | 4.07718 | 0.16142 |
| H | -3.75895 | 2.44219 | 4.42367 |
| H | -0.31361 | 6.68803 | 0.85042 |
| H | -0.70648 | 7.72923 | 4.42367 |
| H | 1.64400 | 6.08311 | 0.16142 |
| H | 0.70648 | 7.72923 | 4.42367 |
| H | 0.50377 | -0.89465 | 8.00480 |
| H | 0.85178 | -1.80640 | 11.33049 |
| H | 3.68377 | -0.89465 | 8.00480 |
| H | 4.03178 | -1.80640 | 11.33049 |
| H | -1.88525 | 5.88875 | 11.33049 |
| H | -0.92162 | 5.73424 | 8.00478 |
| H | 7.73748 | 1.65759 | 11.33051 |
| H | 6.05397 | 1.67045 | 7.37054 |
| H | 4.33096 | 5.73424 | 8.00478 |
| H | 5.29459 | 5.88875 | 11.33049 |

Table 6: $3 \times 3$ $MoSe_2$-$WS_2$

| Atom | X | Y | Z |
|---|---|---|---|
| Mo | 0.00000 | 1.89833 | 4.07000 |
| Mo | -1.64400 | 4.74582 | 4.07000 |
| Mo | -3.28800 | 7.59331 | 4.07000 |
| Mo | 3.28800 | 1.89833 | 4.07000 |
| Mo | 1.64400 | 4.74582 | 4.07000 |
| Mo | 0.00000 | 7.59331 | 4.07000 |
| Mo | 6.57600 | 1.89833 | 4.07000 |
| Mo | 4.93200 | 4.74582 | 4.07000 |
| Mo | 3.28800 | 7.59331 | 4.07000 |
| Se | 1.64400 | 0.94916 | 5.73668 |
| Se | 0.00000 | 3.79665 | 5.73668 |
| Se | -1.64400 | 6.64415 | 5.73668 |
| Se | 4.93200 | 0.94916 | 5.73668 |
| Se | 3.28800 | 3.79665 | 5.73668 |
| Se | 1.64400 | 6.64415 | 5.73668 |
| Se | 8.22000 | 0.94916 | 5.73668 |
| Se | 6.57600 | 3.79665 | 5.73668 |
| Se | 4.93200 | 6.64415 | 5.73668 |
| Se | 1.64400 | 0.94916 | 2.40332 |
| Se | 0.00000 | 3.79665 | 2.40332 |
| Se | -1.64400 | 6.64415 | 2.40332 |
| Se | 4.93200 | 0.94916 | 2.40332 |
| Se | 3.28800 | 3.79665 | 2.40332 |
| Se | 1.64400 | 6.64415 | 2.40332 |
| Se | 8.22000 | 0.94916 | 2.40332 |
| Se | 6.57600 | 3.79665 | 2.40332 |
| Se | 4.93200 | 6.64415 | 2.40332 |
| Se | -1.64400 | 0.94916 | 2.40332 |
| Se | -1.64400 | 0.94916 | 5.73668 |
| Se | -3.28800 | 3.79665 | 2.40332 |
| Se | -3.28800 | 3.79665 | 5.73668 |
| Se | -4.93200 | 6.64415 | 2.40332 |
| Se | -4.93200 | 6.64415 | 5.73668 |
| Se | -3.28800 | 9.49164 | 2.40332 |
| Se | -3.28800 | 9.49164 | 5.73668 |
| Se | 0.00000 | 9.49164 | 2.40332 |
| Se | 0.00000 | 9.49164 | 5.73668 |
| Se | 3.28800 | 9.49164 | 2.40332 |
| Se | 3.28800 | 9.49164 | 5.73668 |
| S | 6.38877 | 7.32729 | 12.60634 |
| S | 6.38877 | 7.32729 | 9.48134 |
| W | 4.79877 | 6.40929 | 11.04384 |
| S | 3.20877 | 7.32729 | 9.48134 |
| S | 3.20877 | 7.32729 | 12.60634 |
| S | 7.97877 | 4.57329 | 9.48134 |
| S | 7.97877 | 4.57329 | 12.60634 |
| W | 1.61877 | 6.40929 | 11.04384 |
| W | 6.38877 | 3.65529 | 11.04384 |
| S | 9.56877 | 1.81939 | 12.60634 |
| S | 9.56877 | 1.81939 | 9.48134 |
| S | 0.02877 | 7.32729 | 12.60634 |
| S | 0.02877 | 7.32729 | 9.48134 |
| S | 4.79877 | 4.57329 | 12.60634 |

| Atom | X | Y | Z |
|---|---|---|---|
| S | 4.79877 | 4.57329 | 9.48134 |
| W | -1.56123 | 6.40929 | 11.04384 |
| W | 3.20877 | 3.65529 | 11.04384 |
| W | 7.97877 | 0.90139 | 11.04384 |
| S | 6.38877 | 1.81939 | 9.48134 |
| S | -3.15123 | 7.32729 | 12.60634 |
| S | 6.38877 | 1.81939 | 12.60634 |
| S | -3.15123 | 7.32729 | 9.48134 |
| S | 1.61877 | 4.57329 | 9.48134 |
| S | 1.61877 | 4.57329 | 12.60634 |
| W | 4.79877 | 0.90139 | 11.04384 |
| W | 0.02877 | 3.65529 | 11.04384 |
| S | 7.97877 | -0.93461 | 12.60634 |
| S | -1.56123 | 4.57329 | 9.48134 |
| S | 3.20877 | 1.81939 | 12.60634 |
| S | -1.56123 | 4.57329 | 12.60634 |
| S | 3.20877 | 1.81939 | 9.48134 |
| S | 7.97877 | -0.93461 | 9.48134 |
| W | 1.61877 | 0.90139 | 11.04384 |
| S | 0.02877 | 1.81939 | 12.60634 |
| S | 0.02877 | 1.81939 | 9.48134 |
| S | 4.79877 | -0.93461 | 12.60634 |
| S | 4.79877 | -0.93461 | 9.48134 |
| S | 1.61877 | -0.93461 | 9.48134 |
| S | 1.61877 | -0.93461 | 12.60634 |
| H | 9.62847 | 1.21854 | 5.26367 |
| H | 8.92320 | 2.07937 | 1.69042 |
| H | -2.34720 | 2.07937 | 1.69042 |
| H | -3.05247 | 1.21854 | 5.26367 |
| H | -3.99120 | 4.92686 | 1.69042 |
| H | -4.69647 | 4.06603 | 5.26367 |
| H | -5.63520 | 7.77436 | 1.69042 |
| H | -6.34047 | 6.91353 | 5.26367 |
| H | -4.61839 | 9.53552 | 1.69042 |
| H | -4.22552 | 10.57672 | 5.26367 |
| H | 1.33039 | 9.53552 | 1.69042 |
| H | 0.93752 | 10.57672 | 5.26367 |
| H | 4.61839 | 9.53552 | 1.69042 |
| H | 4.22552 | 10.57672 | 5.26367 |
| H | 6.79868 | 8.54880 | 12.17102 |
| H | 5.96807 | 7.08439 | 8.21106 |
| H | 8.62598 | 3.56028 | 8.84532 |
| H | 9.24158 | 4.31753 | 12.17103 |
| H | 10.83158 | 1.56363 | 12.17103 |
| H | 10.21598 | 0.80638 | 8.84532 |
| H | -3.56114 | 8.54880 | 12.17102 |
| H | -2.73053 | 7.08439 | 8.21106 |
| H | 8.83166 | -1.90036 | 12.17101 |
| H | 9.17967 | -0.98861 | 8.84532 |
| H | 3.94588 | -1.90036 | 12.17101 |
| H | 4.79877 | -0.44883 | 8.21106 |
| H | 1.61877 | -0.44883 | 8.21106 |
| H | 2.47166 | -1.90036 | 12.17101 |

Table 7: $2 \times 2$ $MoSe_2$-$MoSe_2$

| Atom | X | Y | Z |
|---|---|---|---|
| Mo | 0.00000 | 1.89833 | 3.23000 |
| Mo | -1.64400 | 4.74582 | 3.23000 |
| Mo | 3.28800 | 1.89833 | 3.23000 |
| Mo | 1.64400 | 4.74582 | 3.23000 |
| Mo | 1.64400 | 0.94916 | 9.69000 |
| Mo | 0.00000 | 3.79665 | 9.69000 |
| Mo | 4.93200 | 0.94916 | 9.69000 |
| Mo | 3.28800 | 3.79665 | 9.69000 |
| Se | 0.00000 | 1.89833 | 8.02332 |
| Se | -1.64400 | 4.74582 | 8.02332 |
| Se | 3.28800 | 1.89833 | 8.02332 |
| Se | 1.64400 | 4.74582 | 8.02332 |
| Se | 1.64400 | 0.94916 | 4.89668 |
| Se | 0.00000 | 3.79665 | 4.89668 |
| Se | 4.93200 | 0.94916 | 4.89668 |
| Se | 3.28800 | 3.79665 | 4.89668 |
| Se | 1.64400 | 0.94916 | 1.56332 |
| Se | 0.00000 | 3.79665 | 1.56332 |
| Se | 4.93200 | 0.94916 | 1.56332 |
| Se | 3.28800 | 3.79665 | 1.56332 |
| Se | 0.00000 | 1.89833 | 11.35668 |
| Se | -1.64400 | 4.74582 | 11.35668 |
| Se | 3.28800 | 1.89833 | 11.35668 |
| Se | 1.64400 | 4.74582 | 11.35668 |
| Se | -1.64400 | 0.94916 | 1.56332 |
| Se | -1.64400 | 0.94916 | 4.89668 |
| Se | -3.28800 | 3.79665 | 1.56332 |
| Se | -3.28800 | 3.79665 | 4.89668 |
| Se | -1.64400 | 6.64415 | 1.56332 |
| Se | -1.64400 | 6.64415 | 4.89668 |

| Atom | X | Y | Z |
|---|---|---|---|
| Se | 1.64400 | 6.64415 | 1.56332 |
| Se | 1.64400 | 6.64415 | 4.89668 |
| Se | 1.64400 | -0.94916 | 8.02332 |
| Se | 1.64400 | -0.94916 | 11.35668 |
| Se | 4.93200 | -0.94916 | 8.02332 |
| Se | 4.93200 | -0.94916 | 11.35668 |
| Se | 6.57600 | 1.89833 | 8.02332 |
| Se | 6.57600 | 1.89833 | 11.35668 |
| Se | 4.93200 | 4.74582 | 8.02332 |
| Se | 4.93200 | 4.74582 | 11.35668 |
| H | -1.15812 | 4.46530 | 6.62142 |
| H | 5.40295 | -0.40530 | 4.42367 |
| H | 4.30481 | -0.22493 | 0.85042 |
| H | -3.05247 | 4.47644 | 10.88367 |
| H | -1.01681 | -0.22493 | 0.85042 |
| H | -2.11495 | -0.40530 | 4.42367 |
| H | -3.99120 | 4.92687 | 0.85042 |
| H | -4.69647 | 4.06603 | 4.42367 |
| H | -2.97439 | 6.68803 | 0.85042 |
| H | -2.58152 | 7.72923 | 4.42367 |
| H | 0.31361 | 6.68803 | 0.85042 |
| H | 0.70648 | 7.72923 | 4.42367 |
| H | 1.64400 | -0.38812 | 6.62142 |
| H | 0.70648 | -2.03425 | 10.88367 |
| H | 4.93200 | -0.38812 | 6.62142 |
| H | 3.99448 | -2.03425 | 10.88367 |
| H | 5.94881 | 3.07242 | 7.31042 |
| H | 7.04695 | 3.25279 | 10.88367 |
| H | 4.44612 | 4.46530 | 6.62142 |
| H | 6.34047 | 4.47644 | 10.88367 |

Table 8: $3 \times 3$ $MoSe_2$-$MoSe_2$

| Atom | X | Y | Z |
|---|---|---|---|
| Mo | 0.00000 | 1.89833 | 29.07000 |
| Mo | -1.64400 | 4.74582 | 29.07000 |
| Mo | -3.28800 | 7.59331 | 29.07000 |
| Mo | 3.28800 | 1.89833 | 29.07000 |
| Mo | 1.64400 | 4.74582 | 29.07000 |
| Mo | 0.00000 | 7.59331 | 29.07000 |
| Mo | 6.57600 | 1.89833 | 29.07000 |
| Mo | 4.93200 | 4.74582 | 29.07000 |
| Mo | 3.28800 | 7.59331 | 29.07000 |
| Mo | 1.64400 | 0.94916 | 35.53000 |
| Mo | 0.00000 | 3.79665 | 35.53000 |
| Mo | -1.64400 | 6.64415 | 35.53000 |
| Mo | 4.93200 | 0.94916 | 35.53000 |
| Mo | 3.28800 | 3.79665 | 35.53000 |
| Mo | 1.64400 | 6.64415 | 35.53000 |
| Mo | 8.22000 | 0.94916 | 35.53000 |
| Mo | 6.57600 | 3.79665 | 35.53000 |
| Mo | 4.93200 | 6.64415 | 35.53000 |
| Se | 0.00000 | 1.89833 | 33.86332 |
| Se | -1.64400 | 4.74582 | 33.86332 |
| Se | -3.28800 | 7.59331 | 33.86332 |
| Se | 3.28800 | 1.89833 | 33.86332 |
| Se | 1.64400 | 4.74582 | 33.86332 |
| Se | 0.00000 | 7.59331 | 33.86332 |
| Se | 6.57600 | 1.89833 | 33.86332 |
| Se | 4.93200 | 4.74582 | 33.86332 |
| Se | 3.28800 | 7.59331 | 33.86332 |
| Se | 1.64400 | 0.94916 | 30.73668 |
| Se | 0.00000 | 3.79665 | 30.73668 |
| Se | -1.64400 | 6.64415 | 30.73668 |
| Se | 4.93200 | 0.94916 | 30.73668 |
| Se | 3.28800 | 3.79665 | 30.73668 |
| Se | 1.64400 | 6.64415 | 30.73668 |
| Se | 8.22000 | 0.94916 | 30.73668 |
| Se | 6.57600 | 3.79665 | 30.73668 |
| Se | 4.93200 | 6.64415 | 30.73668 |
| Se | 1.64400 | 0.94916 | 27.40332 |
| Se | 0.00000 | 3.79665 | 27.40332 |
| Se | -1.64400 | 6.64415 | 27.40332 |
| Se | 4.93200 | 0.94916 | 27.40332 |
| Se | 3.28800 | 3.79665 | 27.40332 |
| Se | 1.64400 | 6.64415 | 27.40332 |
| Se | 8.22000 | 0.94916 | 27.40332 |
| Se | 6.57600 | 3.79665 | 27.40332 |
| Se | 4.93200 | 6.64415 | 27.40332 |
| Se | 0.00000 | 1.89833 | 37.19668 |
| Se | -1.64400 | 4.74582 | 37.19668 |
| Se | -3.28800 | 7.59331 | 37.19668 |
| Se | 3.28800 | 1.89833 | 37.19668 |
| Se | 1.64400 | 4.74582 | 37.19668 |
| Se | 0.00000 | 7.59331 | 37.19668 |
| Se | 6.57600 | 1.89833 | 37.19668 |
| Se | 4.93200 | 4.74582 | 37.19668 |

| Atom | X | Y | Z |
|---|---|---|---|
| Se | 3.28800 | 7.59331 | 37.19668 |
| Se | -1.64400 | 0.94916 | 27.40332 |
| Se | -1.64400 | 0.94916 | 30.73668 |
| Se | -3.28800 | 3.79665 | 27.40332 |
| Se | -3.28800 | 3.79665 | 30.73668 |
| Se | -4.93200 | 6.64415 | 27.40332 |
| Se | -4.93200 | 6.64415 | 30.73668 |
| Se | -3.28800 | 9.49164 | 27.40332 |
| Se | -3.28800 | 9.49164 | 30.73668 |
| Se | 0.00000 | 9.49164 | 27.40332 |
| Se | 0.00000 | 9.49164 | 30.73668 |
| Se | 3.28800 | 9.49164 | 27.40332 |
| Se | 3.28800 | 9.49164 | 30.73668 |
| Se | 1.64400 | -0.94916 | 33.86332 |
| Se | 1.64400 | -0.94916 | 37.19668 |
| Se | 4.93200 | -0.94916 | 33.86332 |
| Se | 4.93200 | -0.94916 | 37.19668 |
| Se | 8.22000 | -0.94916 | 33.86332 |
| Se | 8.22000 | -0.94916 | 37.19668 |
| Se | 9.86400 | 1.89833 | 33.86332 |
| Se | 9.86400 | 1.89833 | 37.19668 |
| Se | 8.22000 | 4.74582 | 33.86332 |
| Se | 8.22000 | 4.74582 | 37.19668 |
| Se | 6.57600 | 7.59331 | 33.86332 |
| Se | 6.57600 | 7.59331 | 37.19668 |
| H | -2.80212 | 7.31279 | 32.46142 |
| H | 9.62847 | 1.21854 | 30.26367 |
| H | 8.92320 | 2.07938 | 26.69042 |
| H | -3.75895 | 8.94777 | 36.72367 |
| H | -1.01681 | -0.22493 | 26.69042 |
| H | -2.11495 | -0.40530 | 30.26367 |
| H | -3.99120 | 4.92687 | 26.69042 |
| H | -4.69647 | 4.06603 | 30.26367 |
| H | -5.63520 | 7.77436 | 26.69042 |
| H | -6.34047 | 6.91352 | 30.26367 |
| H | -4.61839 | 9.53552 | 26.69042 |
| H | -4.22552 | 10.57672 | 30.26367 |
| H | -1.33039 | 9.53552 | 26.69042 |
| H | -0.93752 | 10.57672 | 30.26367 |
| H | 4.61839 | 9.53552 | 26.69042 |
| H | 4.22552 | 10.57672 | 30.26367 |
| H | 0.31361 | -0.99305 | 33.15042 |
| H | 0.70648 | -2.03425 | 36.72367 |
| H | 3.60161 | -0.99305 | 33.15042 |
| H | 3.99448 | -2.03425 | 36.72367 |
| H | 6.88961 | -0.99305 | 33.15042 |
| H | 7.28248 | -2.03425 | 36.72367 |
| H | 9.37812 | 1.61781 | 32.46142 |
| H | 10.33495 | 3.25279 | 36.72367 |
| H | 8.92320 | 3.61561 | 33.15042 |
| H | 9.62847 | 4.47644 | 36.72367 |
| H | 6.09012 | 7.31279 | 32.46142 |
| H | 7.98447 | 7.32393 | 36.72367 |

Table 9: $2 \times 2$ $WSe_2$-$WSe_2$

| Atom | X | Y | Z |
|---|---|---|---|
| W | 1.64250 | 0.94830 | 3.24600 |
| W | 0.00000 | 3.79319 | 3.24600 |
| W | 4.92750 | 0.94830 | 3.24600 |
| W | 3.28500 | 3.79319 | 3.24600 |
| W | -0.00000 | 1.89660 | 9.73800 |
| W | -1.64250 | 4.74149 | 9.73800 |
| W | 3.28500 | 1.89660 | 9.73800 |
| W | 1.64250 | 4.74149 | 9.73800 |
| Se | 0.00000 | 1.89660 | 1.55808 |
| Se | -1.64250 | 4.74149 | 1.55808 |
| Se | 3.28500 | 1.89660 | 1.55808 |
| Se | 1.64250 | 4.74149 | 1.55808 |
| Se | 1.64250 | 0.94830 | 11.42592 |
| Se | 0.00000 | 3.79319 | 11.42592 |
| Se | 4.92750 | 0.94830 | 11.42592 |
| Se | 3.28500 | 3.79319 | 11.42592 |
| Se | 1.64250 | 0.94830 | 8.05008 |
| Se | 0.00000 | 3.79319 | 8.05008 |
| Se | 4.92750 | 0.94830 | 8.05008 |
| Se | 3.28500 | 3.79319 | 8.05008 |
| Se | 0.00000 | 1.89660 | 4.93392 |
| Se | -1.64250 | 4.74149 | 4.93392 |
| Se | 3.28500 | 1.89660 | 4.93392 |
| Se | 1.64250 | 4.74149 | 4.93392 |
| Se | 1.64250 | -0.94830 | 1.55808 |
| Se | 1.64250 | -0.94830 | 4.93392 |
| Se | 4.92750 | -0.94830 | 1.55808 |
| Se | 4.92750 | -0.94830 | 4.93392 |
| Se | 6.57000 | 1.89660 | 1.55808 |
| Se | 6.57000 | 1.89660 | 4.93392 |

| Atom | X | Y | Z |
|---|---|---|---|
| Se | 4.92750 | 4.74149 | 1.55808 |
| Se | 4.92750 | 4.74149 | 4.93392 |
| Se | -1.64250 | 0.94830 | 8.05008 |
| Se | -1.64250 | 0.94830 | 11.42592 |
| Se | -3.28500 | 3.79319 | 8.05008 |
| Se | -3.28500 | 3.79319 | 11.42592 |
| Se | -1.64250 | 6.63809 | 8.05008 |
| Se | -1.64250 | 6.63809 | 11.42592 |
| Se | 1.64250 | 6.63809 | 8.05008 |
| Se | 1.64250 | 6.63809 | 11.42592 |
| H | -1.14846 | 4.45625 | 0.15999 |
| H | 6.33872 | 1.21141 | 10.95759 |
| H | 5.62395 | 2.08092 | 7.33437 |
| H | -3.05372 | 4.47837 | 4.46559 |
| H | 1.64250 | -0.37783 | 0.15999 |
| H | 2.57597 | -2.03889 | 4.46559 |
| H | 3.59840 | -0.98513 | 0.84237 |
| H | 3.99403 | -2.03889 | 4.46559 |
| H | 6.07596 | 1.61136 | 0.15999 |
| H | 7.04775 | 3.25030 | 4.46559 |
| H | 4.43346 | 4.45625 | 0.15999 |
| H | 6.33872 | 4.47837 | 4.46559 |
| H | -1.00985 | -0.22115 | 7.33437 |
| H | -2.12025 | -0.40541 | 10.95759 |
| H | -2.79096 | 4.07843 | 6.65199 |
| H | -3.76275 | 2.43948 | 10.95759 |
| H | -0.31340 | 6.67492 | 7.33437 |
| H | -0.70903 | 7.72868 | 10.95759 |
| H | 2.97160 | 6.67492 | 7.33437 |
| H | 2.57597 | 7.72868 | 10.95759 |

Table 10: $3 \times 3$ $WSe_2$-$WSe_2$

| Atom | X | Y | Z |
|---|---|---|---|
| W | 1.64250 | 0.94830 | 3.24600 |
| W | 0.00000 | 3.79319 | 3.24600 |
| W | -1.64250 | 6.63809 | 3.24600 |
| W | 4.92750 | 0.94830 | 3.24600 |
| W | 3.28500 | 3.79319 | 3.24600 |
| W | 1.64250 | 6.63809 | 3.24600 |
| W | 8.21250 | 0.94830 | 3.24600 |
| W | 6.57000 | 3.79319 | 3.24600 |
| W | 4.92750 | 6.63809 | 3.24600 |
| W | -0.00000 | 1.89660 | 9.73800 |
| W | -1.64250 | 4.74149 | 9.73800 |
| W | -3.28500 | 7.58638 | 9.73800 |
| W | 3.28500 | 1.89660 | 9.73800 |
| W | 1.64250 | 4.74149 | 9.73800 |
| W | -0.00000 | 7.58638 | 9.73800 |
| W | 6.57000 | 1.89660 | 9.73800 |
| W | 4.92750 | 4.74149 | 9.73800 |
| W | 3.28500 | 7.58638 | 9.73800 |
| Se | 0.00000 | 1.89660 | 1.55808 |
| Se | -1.64250 | 4.74149 | 1.55808 |
| Se | -3.28500 | 7.58638 | 1.55808 |
| Se | 3.28500 | 1.89660 | 1.55808 |
| Se | 1.64250 | 4.74149 | 1.55808 |
| Se | 0.00000 | 7.58638 | 1.55808 |
| Se | 6.57000 | 1.89660 | 1.55808 |
| Se | 4.92750 | 4.74149 | 1.55808 |
| Se | 3.28500 | 7.58638 | 1.55808 |
| Se | 1.64250 | 0.94830 | 11.42592 |
| Se | 0.00000 | 3.79319 | 11.42592 |
| Se | -1.64250 | 6.63809 | 11.42592 |
| Se | 4.92750 | 0.94830 | 11.42592 |
| Se | 3.28500 | 3.79319 | 11.42592 |
| Se | 1.64250 | 6.63809 | 11.42592 |
| Se | 8.21250 | 0.94830 | 11.42592 |
| Se | 6.57000 | 3.79319 | 11.42592 |
| Se | 4.92750 | 6.63809 | 11.42592 |
| Se | 1.64250 | 0.94830 | 8.05008 |
| Se | 0.00000 | 3.79319 | 8.05008 |
| Se | -1.64250 | 6.63809 | 8.05008 |
| Se | 4.92750 | 0.94830 | 8.05008 |
| Se | 3.28500 | 3.79319 | 8.05008 |
| Se | 1.64250 | 6.63809 | 8.05008 |
| Se | 8.21250 | 0.94830 | 8.05008 |
| Se | 6.57000 | 3.79319 | 8.05008 |
| Se | 4.92750 | 6.63809 | 8.05008 |
| Se | 0.00000 | 1.89660 | 4.93392 |
| Se | -1.64250 | 4.74149 | 4.93392 |
| Se | -3.28500 | 7.58638 | 4.93392 |
| Se | 3.28500 | 1.89660 | 4.93392 |
| Se | 1.64250 | 4.74149 | 4.93392 |
| Se | 0.00000 | 7.58638 | 4.93392 |
| Se | 6.57000 | 1.89660 | 4.93392 |
| Se | 4.92750 | 4.74149 | 4.93392 |
| Se | 3.28500 | 7.58638 | 4.93392 |
| Se | 1.64250 | -0.94830 | 1.55808 |
| Se | 1.64250 | -0.94830 | 4.93392 |
| Se | 4.92750 | -0.94830 | 1.55808 |
| Se | 4.92750 | -0.94830 | 4.93392 |
| Se | 8.21250 | -0.94830 | 1.55808 |
| Se | 8.21250 | -0.94830 | 4.93392 |
| Se | 9.85500 | 1.89660 | 1.55808 |
| Se | 9.85500 | 1.89660 | 4.93392 |
| Se | 8.21250 | 4.74149 | 1.55808 |
| Se | 8.21250 | 4.74149 | 4.93392 |
| Se | 6.57000 | 7.58638 | 1.55808 |
| Se | 6.57000 | 7.58638 | 4.93392 |
| Se | -1.64250 | 0.94830 | 8.05008 |
| Se | -1.64250 | 0.94830 | 11.42592 |
| Se | -3.28500 | 3.79319 | 8.05008 |
| Se | -3.28500 | 3.79319 | 11.42592 |
| Se | -4.92750 | 6.63809 | 8.05008 |
| Se | -4.92750 | 6.63809 | 11.42592 |
| Se | -3.28500 | 9.48298 | 8.05008 |
| Se | -3.28500 | 9.48298 | 11.42592 |
| Se | 0.00000 | 9.48298 | 8.05008 |
| Se | 0.00000 | 9.48298 | 11.42592 |
| Se | 3.28500 | 9.48298 | 8.05008 |
| Se | 3.28500 | 9.48298 | 11.42592 |
| H | -2.65235 | 8.75583 | 0.84237 |
| H | 8.69025 | -0.40541 | 10.95759 |
| H | 7.71846 | 1.23353 | 6.65199 |
| H | -3.76275 | 8.94009 | 4.46559 |
| H | 1.64250 | -0.37783 | 0.15999 |
| H | 2.57597 | -2.03889 | 4.46559 |
| H | 4.92750 | -0.37783 | 0.15999 |
| H | 3.99403 | -2.03889 | 4.46559 |
| H | 6.88340 | -0.98513 | 0.84237 |
| H | 7.27903 | -2.03889 | 4.46559 |
| H | 9.36096 | 1.61136 | 0.15999 |
| H | 10.33275 | 3.25030 | 4.46559 |
| H | 7.71846 | 4.45625 | 0.15999 |
| H | 9.62372 | 4.47837 | 4.46559 |
| H | 7.26645 | 6.45376 | 0.84237 |
| H | 7.98122 | 7.32327 | 4.46559 |
| H | -1.14846 | 1.23353 | 6.65199 |
| H | -3.05372 | 1.21141 | 10.95759 |
| H | -2.79096 | 4.07843 | 6.65199 |
| H | -2.79096 | 4.07843 | 12.82401 |
| H | -4.43346 | 6.92332 | 6.65199 |
| H | -6.33872 | 6.90120 | 10.95759 |
| H | -1.95590 | 9.51981 | 7.33437 |
| H | -2.35153 | 10.57357 | 10.95759 |
| H | 1.32910 | 9.51981 | 7.33437 |
| H | 0.93347 | 10.57357 | 10.95759 |
| H | 3.28500 | 8.91251 | 6.65199 |
| H | 2.35153 | 10.57357 | 10.95759 |

Table 11: $2 \times 2$ $MoS_2$-$MoS_2$

| Atom | X | Y | Z |
|---|---|---|---|
| Mo | 0.00000 | 1.82500 | 3.07375 |
| Mo | -1.58050 | 4.56251 | 3.07375 |
| Mo | 3.16100 | 1.82500 | 3.07375 |
| Mo | 1.58050 | 4.56251 | 3.07375 |
| Mo | 1.58050 | 0.91250 | 9.22125 |
| Mo | 0.00000 | 3.65001 | 9.22125 |
| Mo | 4.74150 | 0.91250 | 9.22125 |
| Mo | 3.16100 | 3.65001 | 9.22125 |
| S | 0.00000 | 1.82500 | 7.71511 |
| S | -1.58050 | 4.56251 | 7.71511 |
| S | 3.16100 | 1.82500 | 7.71511 |
| S | 1.58050 | 4.56251 | 7.71511 |
| S | 1.58050 | 0.91250 | 4.57989 |
| S | 0.00000 | 3.65001 | 4.57989 |
| S | 4.74150 | 0.91250 | 4.57989 |
| S | 3.16100 | 3.65001 | 4.57989 |
| S | 1.58050 | 0.91250 | 1.56761 |
| S | 0.00000 | 3.65001 | 1.56761 |
| S | 4.74150 | 0.91250 | 1.56761 |
| S | 3.16100 | 3.65001 | 1.56761 |
| S | 0.00000 | 1.82500 | 10.72739 |
| S | -1.58050 | 4.56251 | 10.72739 |
| S | 3.16100 | 1.82500 | 10.72739 |
| S | 1.58050 | 4.56251 | 10.72739 |
| S | -1.58050 | 0.91250 | 1.56761 |
| S | -1.58050 | 0.91250 | 4.57989 |
| S | -3.16100 | 3.65001 | 1.56761 |
| S | -3.16100 | 3.65001 | 4.57989 |
| S | -1.58050 | 6.38751 | 1.56761 |
| S | -1.58050 | 6.38751 | 4.57989 |

| Atom | X | Y | Z |
|---|---|---|---|
| S | 1.58050 | 6.38751 | 1.56761 |
| S | 1.58050 | 6.38751 | 4.57989 |
| S | 1.58050 | -0.91250 | 7.71511 |
| S | 1.58050 | -0.91250 | 10.72739 |
| S | 4.74150 | -0.91250 | 7.71511 |
| S | 4.74150 | -0.91250 | 10.72739 |
| S | 6.32200 | 1.82500 | 7.71511 |
| S | 6.32200 | 1.82500 | 10.72739 |
| S | 4.74150 | 4.56251 | 7.71511 |
| S | 4.74150 | 4.56251 | 10.72739 |
| H | -1.17649 | 4.32926 | 6.43763 |
| H | 5.13709 | -0.31062 | 4.13594 |
| H | 4.19873 | -0.16384 | 0.93794 |
| H | -2.83755 | 4.29354 | 10.28344 |
| H | -1.03773 | -0.16384 | 0.93794 |
| H | -1.97609 | -0.31062 | 4.13594 |
| H | -3.82176 | 4.65823 | 0.93794 |
| H | -4.41805 | 3.91898 | 4.13594 |
| H | -2.78403 | 6.45563 | 0.93794 |
| H | -2.44196 | 7.34167 | 4.13594 |
| H | 0.37697 | 6.45563 | 0.93794 |
| H | 0.71904 | 7.34167 | 4.13594 |
| H | 1.58050 | -0.44599 | 6.43763 |
| H | 0.71904 | -1.86665 | 10.28344 |
| H | 4.74150 | -0.44599 | 6.43763 |
| H | 5.60296 | -1.86665 | 10.28344 |
| H | 5.77923 | 2.90135 | 7.08544 |
| H | 6.71759 | 3.04812 | 10.28344 |
| H | 4.33749 | 4.32926 | 6.43763 |
| H | 5.99855 | 4.29354 | 10.28344 |

Table 12: $3 \times 3$ $MoS_2$-$MoS_2$

| Atom | X | Y | Z |
|---|---|---|---|
| Mo | 0.00000 | 1.82500 | 27.66375 |
| Mo | -1.58050 | 4.56251 | 27.66375 |
| Mo | -3.16100 | 7.30002 | 27.66375 |
| Mo | 3.16100 | 1.82500 | 27.66375 |
| Mo | 1.58050 | 4.56251 | 27.66375 |
| Mo | 0.00000 | 7.30002 | 27.66375 |
| Mo | 6.32200 | 1.82500 | 27.66375 |
| Mo | 4.74150 | 4.56251 | 27.66375 |
| Mo | 3.16100 | 7.30002 | 27.66375 |
| Mo | 1.58050 | 0.91250 | 33.81125 |
| Mo | 0.00000 | 3.65001 | 33.81125 |
| Mo | -1.58050 | 6.38751 | 33.81125 |
| Mo | 4.74150 | 0.91250 | 33.81125 |
| Mo | 3.16100 | 3.65001 | 33.81125 |
| Mo | 1.58050 | 6.38751 | 33.81125 |
| Mo | 7.90250 | 0.91250 | 33.81125 |
| Mo | 6.32200 | 3.65001 | 33.81125 |
| Mo | 4.74150 | 6.38751 | 33.81125 |
| S | 0.00000 | 1.82500 | 32.30511 |
| S | -1.58050 | 4.56251 | 32.30511 |
| S | -3.16100 | 7.30002 | 32.30511 |
| S | 3.16100 | 1.82500 | 32.30511 |
| S | 1.58050 | 4.56251 | 32.30511 |
| S | 0.00000 | 7.30002 | 32.30511 |
| S | 6.32200 | 1.82500 | 32.30511 |
| S | 4.74150 | 4.56251 | 32.30511 |
| S | 3.16100 | 7.30002 | 32.30511 |
| S | 1.58050 | 0.91250 | 29.16989 |
| S | 0.00000 | 3.65001 | 29.16989 |
| S | -1.58050 | 6.38751 | 29.16989 |
| S | 4.74150 | 0.91250 | 29.16989 |
| S | 3.16100 | 3.65001 | 29.16989 |
| S | 1.58050 | 6.38751 | 29.16989 |
| S | 7.90250 | 0.91250 | 29.16989 |
| S | 6.32200 | 3.65001 | 29.16989 |
| S | 4.74150 | 6.38751 | 29.16989 |
| S | 1.58050 | 0.91250 | 26.15761 |
| S | 0.00000 | 3.65001 | 26.15761 |
| S | -1.58050 | 6.38751 | 26.15761 |
| S | 4.74150 | 0.91250 | 26.15761 |
| S | 3.16100 | 3.65001 | 26.15761 |
| S | 1.58050 | 6.38751 | 26.15761 |
| S | 7.90250 | 0.91250 | 26.15761 |
| S | 6.32200 | 3.65001 | 26.15761 |
| S | 4.74150 | 6.38751 | 26.15761 |
| S | 0.00000 | 1.82500 | 35.31739 |
| S | -1.58050 | 4.56251 | 35.31739 |
| S | -3.16100 | 7.30002 | 35.31739 |
| S | 3.16100 | 1.82500 | 35.31739 |
| S | 1.58050 | 4.56251 | 35.31739 |
| S | 0.00000 | 7.30002 | 35.31739 |
| S | 6.32200 | 1.82500 | 35.31739 |
| S | 4.74150 | 4.56251 | 35.31739 |

| Atom | X | Y | Z |
|---|---|---|---|
| S | 3.16100 | 7.30002 | 35.31739 |
| S | -1.58050 | 0.91250 | 26.15761 |
| S | -1.58050 | 0.91250 | 29.16989 |
| S | -3.16100 | 3.65001 | 26.15761 |
| S | -3.16100 | 3.65001 | 29.16989 |
| S | -4.74150 | 6.38751 | 26.15761 |
| S | -4.74150 | 6.38751 | 29.16989 |
| S | -3.16100 | 9.12502 | 26.15761 |
| S | -3.16100 | 9.12502 | 29.16989 |
| S | 0.00000 | 9.12502 | 26.15761 |
| S | 0.00000 | 9.12502 | 29.16989 |
| S | 3.16100 | 9.12502 | 26.15761 |
| S | 3.16100 | 9.12502 | 29.16989 |
| S | 1.58050 | -0.91250 | 32.30511 |
| S | 1.58050 | -0.91250 | 35.31739 |
| S | 4.74150 | -0.91250 | 32.30511 |
| S | 4.74150 | -0.91250 | 35.31739 |
| S | 7.90250 | -0.91250 | 32.30511 |
| S | 7.90250 | -0.91250 | 35.31739 |
| S | 9.48300 | 1.82500 | 32.30511 |
| S | 9.48300 | 1.82500 | 35.31739 |
| S | 7.90250 | 4.56251 | 32.30511 |
| S | 7.90250 | 4.56251 | 35.31739 |
| S | 6.32200 | 7.30002 | 32.30511 |
| S | 6.32200 | 7.30002 | 35.31739 |
| H | -2.75699 | 7.06676 | 31.02763 |
| H | 9.15955 | 1.18147 | 28.72594 |
| H | 8.56326 | 1.92073 | 25.52794 |
| H | -3.55659 | 8.52314 | 34.87344 |
| H | -1.03773 | -0.16384 | 25.52794 |
| H | -1.97609 | -0.31062 | 28.72594 |
| H | -2.61823 | 2.57366 | 25.52794 |
| H | -3.55659 | 2.42689 | 28.72594 |
| H | -5.40226 | 7.39574 | 25.52794 |
| H | -5.99855 | 6.65648 | 28.72594 |
| H | -4.36453 | 9.19314 | 25.52794 |
| H | -4.02246 | 10.07917 | 28.72594 |
| H | -1.20353 | 9.19314 | 25.52794 |
| H | -0.86146 | 10.07917 | 28.72594 |
| H | 4.36453 | 9.19314 | 25.52794 |
| H | 4.02246 | 10.07917 | 28.72594 |
| H | 0.37697 | -0.98062 | 31.67544 |
| H | 0.71904 | -1.86665 | 34.87344 |
| H | 5.94503 | -0.98062 | 31.67544 |
| H | 5.60296 | -1.86665 | 34.87344 |
| H | 9.10603 | -0.98062 | 31.67544 |
| H | 8.76396 | -1.86665 | 34.87344 |
| H | 10.14376 | 0.81678 | 31.67544 |
| H | 10.74005 | 1.55604 | 34.87344 |
| H | 8.56326 | 3.55429 | 31.67544 |
| H | 9.15955 | 4.29354 | 34.87344 |
| H | 5.91799 | 7.06676 | 31.02763 |
| H | 6.71759 | 8.52314 | 34.87344 |

Table 13: $2 \times 2$ $WS_2$-$WS_2$

| Atom | X | Y | Z |
|---|---|---|---|
| W | 1.59000 | 0.91799 | 3.12500 |
| W | 0.00000 | 3.67195 | 3.12500 |
| W | 4.77000 | 0.91799 | 3.12500 |
| W | 3.18000 | 3.67195 | 3.12500 |
| W | -0.00000 | 1.83597 | 9.37500 |
| W | -1.59000 | 4.58993 | 9.37500 |
| W | 3.18000 | 1.83597 | 9.37500 |
| W | 1.59000 | 4.58993 | 9.37500 |
| S | 0.00000 | 1.83597 | 4.68750 |
| S | -1.59000 | 4.58993 | 4.68750 |
| S | 3.18000 | 1.83597 | 4.68750 |
| S | 1.59000 | 4.58993 | 4.68750 |
| S | 1.59000 | 0.91799 | 7.81250 |
| S | 0.00000 | 3.67195 | 7.81250 |
| S | 4.77000 | 0.91799 | 7.81250 |
| S | 3.18000 | 3.67195 | 7.81250 |
| S | 1.59000 | 0.91799 | 10.93750 |
| S | 0.00000 | 3.67195 | 10.93750 |
| S | 4.77000 | 0.91799 | 10.93750 |
| S | 3.18000 | 3.67195 | 10.93750 |
| S | 0.00000 | 1.83597 | 1.56250 |
| S | -1.59000 | 4.58993 | 1.56250 |
| S | 3.18000 | 1.83597 | 1.56250 |
| S | 1.59000 | 4.58993 | 1.56250 |
| S | 1.59000 | -0.91799 | 1.56250 |
| S | 1.59000 | -0.91799 | 4.68750 |
| S | 4.77000 | -0.91799 | 1.56250 |
| S | 4.77000 | -0.91799 | 4.68750 |
| S | 6.36000 | 1.83597 | 1.56250 |
| S | 6.36000 | 1.83597 | 4.68750 |

| Atom | X | Y | Z |
|---|---|---|---|
| S | 4.77000 | 4.58993 | 1.56250 |
| S | 4.77000 | 4.58993 | 4.68750 |
| S | -1.59000 | 0.91799 | 7.81250 |
| S | -1.59000 | 0.91799 | 10.93750 |
| S | -3.18000 | 3.67195 | 7.81250 |
| S | -3.18000 | 3.67195 | 10.93750 |
| S | -1.59000 | 6.42591 | 7.81250 |
| S | -1.59000 | 6.42591 | 10.93750 |
| S | 1.59000 | 6.42591 | 7.81250 |
| S | 1.59000 | 6.42591 | 10.93750 |
| H | -2.85281 | 4.33418 | 4.25218 |
| H | 4.21631 | -0.14902 | 7.17648 |
| H | 5.17992 | -0.30352 | 10.50218 |
| H | -1.16929 | 4.34704 | 0.29222 |
| H | 1.59000 | -0.43219 | 0.29222 |
| H | 0.73711 | -1.88374 | 4.25218 |
| H | 3.56910 | -0.97198 | 0.92648 |
| H | 3.91711 | -1.88374 | 4.25218 |
| H | 5.93929 | 1.59308 | 0.29222 |
| H | 6.76992 | 3.05748 | 4.25218 |
| H | 4.34929 | 4.34704 | 0.29222 |
| H | 5.17992 | 5.81144 | 4.25218 |
| H | -1.16929 | 1.16088 | 6.54222 |
| H | -2.85281 | 1.17374 | 10.50218 |
| H | -2.62631 | 2.60494 | 7.17648 |
| H | -3.58992 | 2.45045 | 10.50218 |
| H | -1.59000 | 5.94012 | 6.54222 |
| H | -2.44289 | 7.39166 | 10.50218 |
| H | 1.59000 | 5.94012 | 6.54222 |
| H | 0.73711 | 7.39166 | 10.50218 |

Table 14: $3 \times 3$ $WS_2$-$WS_2$

| Atom | X | Y | Z |
|---|---|---|---|
| W | 1.59000 | 0.91799 | 28.12500 |
| W | 0.00000 | 3.67195 | 28.12500 |
| W | -1.59000 | 6.42591 | 28.12500 |
| W | 4.77000 | 0.91799 | 28.12500 |
| W | 3.18000 | 3.67195 | 28.12500 |
| W | 1.59000 | 6.42591 | 28.12500 |
| W | 7.95000 | 0.91799 | 28.12500 |
| W | 6.36000 | 3.67195 | 28.12500 |
| W | 4.77000 | 6.42591 | 28.12500 |
| W | -0.00000 | 1.83597 | 34.37500 |
| W | -1.59000 | 4.58993 | 34.37500 |
| W | -3.18000 | 7.34390 | 34.37500 |
| W | 3.18000 | 1.83597 | 34.37500 |
| W | 1.59000 | 4.58993 | 34.37500 |
| W | -0.00000 | 7.34390 | 34.37500 |
| W | 6.36000 | 1.83597 | 34.37500 |
| W | 4.77000 | 4.58993 | 34.37500 |
| W | 3.18000 | 7.34390 | 34.37500 |
| S | 0.00000 | 1.83597 | 29.68750 |
| S | -1.59000 | 4.58993 | 29.68750 |
| S | -3.18000 | 7.34390 | 29.68750 |
| S | 3.18000 | 1.83597 | 29.68750 |
| S | 1.59000 | 4.58993 | 29.68750 |
| S | 0.00000 | 7.34390 | 29.68750 |
| S | 6.36000 | 1.83597 | 29.68750 |
| S | 4.77000 | 4.58993 | 29.68750 |
| S | 3.18000 | 7.34390 | 29.68750 |
| S | 1.59000 | 0.91799 | 32.81250 |
| S | 0.00000 | 3.67195 | 32.81250 |
| S | -1.59000 | 6.42591 | 32.81250 |
| S | 4.77000 | 0.91799 | 32.81250 |
| S | 3.18000 | 3.67195 | 32.81250 |
| S | 1.59000 | 6.42591 | 32.81250 |
| S | 7.95000 | 0.91799 | 32.81250 |
| S | 6.36000 | 3.67195 | 32.81250 |
| S | 4.77000 | 6.42591 | 32.81250 |
| S | 1.59000 | 0.91799 | 35.93750 |
| S | 0.00000 | 3.67195 | 35.93750 |
| S | -1.59000 | 6.42591 | 35.93750 |
| S | 4.77000 | 0.91799 | 35.93750 |
| S | 3.18000 | 3.67195 | 35.93750 |
| S | 1.59000 | 6.42591 | 35.93750 |
| S | 7.95000 | 0.91799 | 35.93750 |
| S | 6.36000 | 3.67195 | 35.93750 |
| S | 4.77000 | 6.42591 | 35.93750 |
| S | 0.00000 | 1.83597 | 26.56250 |
| S | -1.59000 | 4.58993 | 26.56250 |
| S | -3.18000 | 7.34390 | 26.56250 |
| S | 3.18000 | 1.83597 | 26.56250 |
| S | 1.59000 | 4.58993 | 26.56250 |
| S | 0.00000 | 7.34390 | 26.56250 |
| S | 6.36000 | 1.83597 | 26.56250 |
| S | 4.77000 | 4.58993 | 26.56250 |
| S | 3.18000 | 7.34390 | 26.56250 |
| S | 1.59000 | -0.91799 | 26.56250 |
| S | 1.59000 | -0.91799 | 29.68750 |
| S | 4.77000 | -0.91799 | 26.56250 |
| S | 4.77000 | -0.91799 | 29.68750 |
| S | 7.95000 | -0.91799 | 26.56250 |
| S | 7.95000 | -0.91799 | 29.68750 |
| S | 9.54000 | 1.83597 | 26.56250 |
| S | 9.54000 | 1.83597 | 29.68750 |
| S | 7.95000 | 4.58993 | 26.56250 |
| S | 7.95000 | 4.58993 | 29.68750 |
| S | 6.36000 | 7.34390 | 26.56250 |
| S | 6.36000 | 7.34390 | 29.68750 |
| S | -1.59000 | 0.91799 | 32.81250 |
| S | -1.59000 | 0.91799 | 35.93750 |
| S | -3.18000 | 3.67195 | 32.81250 |
| S | -3.18000 | 3.67195 | 35.93750 |
| S | -4.77000 | 6.42591 | 32.81250 |
| S | -4.77000 | 6.42591 | 35.93750 |
| S | -3.18000 | 9.17987 | 32.81250 |
| S | -3.18000 | 9.17987 | 35.93750 |
| S | 0.00000 | 9.17987 | 32.81250 |
| S | 0.00000 | 9.17987 | 35.93750 |
| S | 3.18000 | 9.17987 | 32.81250 |
| S | 3.18000 | 9.17987 | 35.93750 |
| H | -3.58992 | 8.56540 | 29.25218 |
| H | 8.59721 | 1.93100 | 32.17648 |
| H | 9.21281 | 1.17374 | 35.50218 |
| H | -2.75929 | 7.10100 | 25.29222 |
| H | 0.38910 | -0.97198 | 25.92648 |
| H | 0.73711 | -1.88374 | 29.25218 |
| H | 4.77000 | -0.43219 | 25.29222 |
| H | 5.62289 | -1.88374 | 29.25218 |
| H | 7.95000 | -0.43219 | 25.29222 |
| H | 8.80289 | -1.88374 | 29.25218 |
| H | 8.98631 | 2.90298 | 25.92648 |
| H | 9.94992 | 3.05748 | 29.25218 |
| H | 7.52929 | 4.34704 | 25.29222 |
| H | 8.35992 | 5.81144 | 29.25218 |
| H | 5.93929 | 7.10100 | 25.29222 |
| H | 7.62281 | 7.08814 | 29.25218 |
| H | -1.03631 | -0.14902 | 32.17648 |
| H | -1.99992 | -0.30352 | 35.50218 |
| H | -3.82721 | 4.68496 | 32.17648 |
| H | -4.44281 | 3.92770 | 35.50218 |
| H | -5.41721 | 7.43892 | 32.17648 |
| H | -6.03281 | 6.68166 | 35.50218 |
| H | -4.38090 | 9.23386 | 32.17648 |
| H | -4.03289 | 10.14562 | 35.50218 |
| H | 1.20090 | 9.23386 | 32.17648 |
| H | 0.85289 | 10.14562 | 35.50218 |
| H | 3.18000 | 8.69408 | 31.54222 |
| H | 2.32711 | 10.14562 | 35.50218 |
